# Supplementary material for: The Large Core of College Admission Markets: Theory and Evidence
Source: arXiv:2010.08631 source file (2022-08-01)
Supplement: Supplementary file 1 [file Appendix_Table_ROLDescriptives_Robust1.tex]

\begin{tabular}{l S[table-number-alignment = center-decimal-marker] S[table-number-alignment = center-decimal-marker] S[table-number-alignment = center-decimal-marker] S[table-number-alignment = center-decimal-marker] S[table-number-alignment = center-decimal-marker]} \\ \hline\hline
 & \multicolumn{1}{c}{{\parbox{2.1cm}{\centering All applicants (\%)}}} & \multicolumn{1}{c}{Capital (\%)} & \multicolumn{1}{c}{County town (\%)} & \multicolumn{1}{c}{Town (\%)} & \multicolumn{1}{c}{Village (\%)} \\ 
 & \multicolumn{1}{c}{(1)} & \multicolumn{1}{c}{(2)} & \multicolumn{1}{c}{(3)} & \multicolumn{1}{c}{(4)} & \multicolumn{1}{c}{(5)} \\ \hline
 \multicolumn{6}{l}{A. {\it Preference for funding}} \\ 
 State-funded contract exclusively & 51.4 & 37.1 & 52.5 & 54.3 & 58.2 \\ 
 Self-funded contract exclusively & 18.5 & 24.0 & 18.8 & 17.5 & 15.2 \\ 
 \multicolumn{6}{c}{} \\ 
 \multicolumn{6}{l}{B. {\it Preference for study characteristics}} \\ 
 Single field of study & 54.9 & 58.9 & 55.2 & 54.1 & 52.4 \\ 
 Single major & 29.6 & 33.5 & 30.5 & 28.7 & 26.9 \\ 
 Same study program consequtively & 15.5 & 20.5 & 14.6 & 14.3 & 13.5 \\ 
 Same study program consequtively on the top of the ROL & 11.6 & 15.0 & 11.3 & 10.7 & 10.2 \\ 
 \multicolumn{5}{c}{} \\ 
 \multicolumn{5}{l}{C. {\it Preference for institution characteristics}} \\ 
 Single program location & 49.4 & 64.5 & 50.0 & 44.4 & 43.5 \\ 
 Single university & 35.0 & 28.8 & 43.2 & 33.7 & 34.7 \\ 
 Single faculty & 26.3 & 24.4 & 30.4 & 25.2 & 25.8 \\ 
\hline \# of applicants & \multicolumn{1}{c}{     108,854} & \multicolumn{1}{c}{      21,731} & \multicolumn{1}{c}{      22,381} & \multicolumn{1}{c}{      35,290} & \multicolumn{1}{c}{      27,532} \\ 
\hline\hline \multicolumn{6}{p{21cm}}{{\it Notes}: The table reports summary statistics on applicants' ROL. Panel A shows the share of applicants who rank state-funded (self-funded) contracts exclusively. Panel B shows the share of applicants who rank exclusively contracts in a single field of study, and in a single major. Panel B also shows the share of applicants who rank the same study program with state-funding and self-funding consequtively, and who rank the same study program with state-funding and self-funding consequtively on the top of the ROL. Panel C shows the share of applicants who rank exclusively contracts that are in the same settlement (single location), at a single university (single university), and at a single faculty of a university (single university). Column (1) presents these shares for all applicants, and columns (2)--(5) report these shares for applicants residing in the capital, county towns, towns, and villages, respectively.}\end{tabular}
